# Supplementary material for: Finding Top-r Influential Communities under Aggregation Functions
Source: arXiv:2207.01029 source file (2022-07-03)
Supplement: Supplementary file 1 [file appendix.tex]

\newpage
\section{Appendix}

\subsection{Additional Applications}
\noindent \textit{\underline{(4) Cocktail Party.}} We aim to plan a successful cocktail party~\cite{haykin2005cocktail,mcdermott2009cocktail,conway2001cocktail}. However, the size of the party is limited. Thus, we want a size-constraint dense subgraph and the influence value of the subgraph is maximum. Considering this, we could assign an influence value of each vertex in the graph, and identify a size-constraint influential community. The influence value of the community is calculated by the sum of influence values of all vertices in the community.

\noindent \textit{\underline{(5) Team Formation~\cite{anagnostopoulos2012online}.}} Given a social network with weighted vertices, the weight indicates each vertex's capability. We are looking for a subgraph where their abilities are high and their cooperation is excellent. Additionally, the size of the subgraph is constrained. For example, a basketball team cannot exceed $15$ players, whereas a soccer team cannot exceed $24$ members. Furthermore, it is not uncommon for us to establish more than one team to attend the contest. Also, there should not exist overlaps between any two teams.

\subsection{Additional Experiments}

\rev{In the case study, as for the top $1$ result set, the $avg$ and $sum$ is the same. As for $min$, ``David J. DeWitt", ``Rakesh Agrawal", and ``H.V Jagadish" are in its result set, while ``Jim Gray" and ``Hamid Piranesh" are in the $avg$ and $sum$ result sets. It is observed that i-10 index of $min$ is significantly larger than $sum$ and $avg$. As for $sum$ and $avg$, the top-$2$ results are almost the same except ``Kyu-Young Whang". Compared with other results, ``Kyu-Young Whang" has fewer citations, H-index, G-index, and i-10 index. Thus, it is observed that $sum$ prefers to discover more diversified research groups, while $avg$ could discover a communties with higher G-index.}
\begin{table}[!ht]
    \centering
    \scalebox{0.9}{

    \begin{tabular}{|l|l|l|l|l|l|}
    \hline
        ~ & \#paper & \#citation & H-Index & G-Index & i-10 \\ \hline
        Michael Stonebraker & 534 & 42173 & 98 & 200 & - \\ \hline
        Michael J. Carey & 447 & 23637 & 81 & 148 & 195 \\ \hline
        David J. DeWitt & 428 & 41844 & 99 & 203 & 178 \\ \hline
        H.V. Jagadish & 687 & 36540 & 89 & 183 & 306 \\ \hline
        Rakesh Agrawal & 542 & 124039 & 103 & 351 & 303 \\ \hline
        Michael J. Franklin & 411 & 65161 & 109 & 254 & 55 \\ \hline
        Hector Garcia Molina & 748 & 102226 & 149 & 313 & 437 \\ \hline
        Hamid Pirahesh & 117 & 13114 & 46 & 114 & 73 \\ \hline
        Jim Gray & 279 & 52829 & 83 & 229 & 167 \\ \hline
        Calvin R. Maurer Jr. & 28 & 3671 & 19 & 28 & - \\ \hline
        Paul Suetens & 401 & 14510 & 53 & 116 & 270 \\ \hline
        Max A. Viergever & 589 & 32589 & 71 & 176 & 518 \\ \hline
        Derek L. G. Hill & 286 & 14614 & 53 & 120 & 501 \\ \hline
        David J. Hawkes & 45 & 2095 & 20 & 45 & 22 \\ \hline
        Christian S. Jensen & 854 & 34946 & 93 & 171 & 364 \\ \hline
        Jennifer Widom & 383 & 62316 & 109 & 249 & 208 \\ \hline
        Richard T. Snodgrass & 322 & 14164 & 56 & 116 & 167 \\ \hline
        Philip A. Bernstein & 347 & 36099 & 77 & 189 & 199 \\ \hline
        M. Tamer Ozsu & 462 & 27183 & 64 & 162 & 183 \\ \hline
        Kyu-Young Whang & 200 & 5176 & 32 & 69 & 71 \\ \hline
        Vimla L. Patel & 364 & 16109 & 69 & 122 & 272 \\ \hline
        Robert A. Greenes & 173 & 4557 & 30 & 66 & - \\ \hline
        Mario Stefanelli & 147 & 2841 & 29 & 51 & - \\ \hline
        Edward H. Shortliffe & 29 & 5572 & 20 & 29 & 210 \\ \hline
        David B. Lomet & 183 & 4920 & 43 & 66 & - \\ \hline
        Guy M. Lohman & 173 & 12199 & 59 & 110 & 117 \\ \hline
        Kenneth A. Ross & 315 & 11266 & 51 & 103 & 122 \\ \hline
        Patrick Valduriez & 569 & 19296 & 55 & 133 & 210 \\ \hline
        Timos K. Sellis & 405 & 17047 & 55 & 125 & 197 \\ \hline
        Graeme P. Penney & 106 & 3695 & 26 & 60 & - \\ \hline
    \end{tabular}
    }
    \caption{Details of each author in the case study. The data is obtained from Aminer.}
	\label{tab:details_case}
\end{table}

    \begin{table}[htbp]
        \centering
        \begin{tabular}{|c|c|c|c|c|} \hline
            \diagbox{Methods}{r} &  5     & 10      & 15     & 20  \\ \hline
             naive                  & 1      &  1     &  1     & 1      \\ \hline
             improved                  & 1  &  1     &  1     & 1      \\ \hline
             greedy                 & 0.9352      &  0.9213     &  0.9019     & 0.8736      \\ \hline
             approx                 & 0.9999607&  0.999877   &  0.999838 & 0.9998048      \\ \hline

        \end{tabular}
        \caption{The NDCG of different algorithms on DomainPub when $k = 6, \epsilon = 0.1$.}
        \label{tab:DP_ndcg}
    \end{table}
    
\rev{\textbf{Quality Comparison for size unconstrained $sum$.}~It is shown in  Table~\ref{tab:DP_ndcg} that NDCG of $approx$ method is nearly exact. As for the $greedy$ algorithm, it could also achieve about high NDCG. When $r$ grows, the NDCG value decreases for all the algorithm.}

    \begin{table}[htbp]
        \centering
        \begin{tabular}{|c|c|c|c|c|} \hline
            \diagbox{k}{r} & 5      & 10        & 15     & 20  \\ \hline
             4             & 1      &  0.9999895  &  0.9999886& 0.99991372  \\ \hline
             6             & 0.9999607&  0.999877   &  0.999838 & 0.9998048      \\ \hline
             8             & 0.999240 &  0.999658   &  0.999653 & 0.999403     \\ \hline
             10            & 0.99722  &  0.99835    &  0.99880  & 0.99867      \\ \hline

        \end{tabular}
        \caption{The NDCG of $approx$ on DomainPub when $\epsilon = 0.1$.}
        \label{tab:approx_ndcg}
    \end{table}
\rev{\textbf{Quality Comparison of $approx$}. Table~\ref{tab:approx_ndcg} illustrates the quality of $approx$ when varying $k$ and $r$. The overall trend of these two parameters is that when $k$ or $r$ grows, the quality of $approx$ decreases. Table~\ref{tab:approx_epsilon_ndcg} shows that result quality when varying $k$ and $\epsilon$. What stands out in this table is that when $\epsilon$ grows, the NDCG of $approx$ would decrease.}

    \begin{table}[htbp]
        \centering
        \begin{tabular}{|c|c|c|c|c|} \hline
            \diagbox{$\epsilon$}{k} & 4      & 6        &  8    & 10  \\ \hline
             0.01           & 1        &  1  &  1 & 1  \\ \hline
             0.1            & 0.9999137&  0.9998048  &  0.999403 & 0.99867      \\ \hline
             0.2            & 0.979240 &  0.96965    &  0.9653  & 0.94108     \\ \hline
             0.3            & 0.97722  &  0.96835    &  0.96480  & 0.93867      \\ \hline
             0.5            & 0.90722  &  0.89835    &  0.88045  & 0.85867      \\ \hline
             0.8            & 0.89722  &  0.86835    &  0.85880  & 0.83867      \\ \hline

        \end{tabular}
        \caption{The NDCG of $approx$ on DomainPub when $r = 20$ by varying k and $\epsilon$.}
        \label{tab:approx_epsilon_ndcg}
    \end{table}

\rev{As for $avg$, we conduct experiments on small dataset, and then $naive$, $improved$, $local search$ ($greedy$) are compared.
\textbf{Quality Comparison of $local search$.}~Both effectiveness and efficiency are compared in the Table~\ref{tab:ls_ndcg} and~\ref{tab:ls_runtime}, respectively. It is shown that $local$ $search$ ($greedy$) could return feasible result.} 
\begin{table}[htbp]
        \centering
        \begin{tabular}{|c|c|c|c|c|} \hline
            \diagbox{Algorithms}{r} &  5     & 10      & 15     & 20  \\ \hline
             naive                  & 1      &  1     &  1     & 1      \\ \hline
             improved                 & 0.8078  &  0.6750     &  0.5732     & 0.5081      \\ \hline
             greedy                 & 0.8863      &  0.8389     &  0.8039     & 0.7782      \\ \hline
             %approx                 & 1      &  1     &  1     & 1      \\ \hline

        \end{tabular}
        \caption{The NDCG of $avg$ on DomainPub when $k = 6$ and $\epsilon = 0.8$.}
        \label{tab:ls_ndcg}
    \end{table}

    \begin{table}[htbp]
        \centering
        \begin{tabular}{|c|c|c|c|c|} \hline
            \diagbox{Algorithms}{r} &  5     & 10      & 15     & 20  \\ \hline
             exact                  & 4.32  &  4.31 &  4.16     & 4.15      \\ \hline
             improved                  & 1.93  &  1.94     &  1.92     & 1.95      \\ \hline
             greedy                 & 0.64  &  0.61     &  0.6     & 0.58      \\ \hline
             %approx                 & 1      &  1     &  1     & 1      \\ \hline

        \end{tabular}
        \caption{The runtime of $approx$ on DomainPub when $k = 6$.}
        \label{tab:ls_runtime}
    \end{table}

\rev{\textbf{Varying Aggregate Functions.}~We also compare the effectiveness and efficiency of $exact$, $improved$, $greedy$ ($local$ $search$), and $random$. Tables~\ref{tab:dagg_ndcg}
 and Table~\ref{tab:dagg_runtime} illustrate the NDCG and runtime. It could be observed that our $greedy$ algorithm could return a feasible result set (at least $0.5737$). As for the efficiency, the $greedy$ is almost the fastest one among all the algorithms.}
 \begin{table}[htbp]
        \centering
        \begin{tabular}{|c|c|c|c|c|} \hline
            \diagbox{functions}{methods} &  exact     & improved      & greedy     & random  \\ \hline
             avg                 & 1      &  0.5081  &  0.7782  & 0.15      \\ \hline
             sum                 & 1      &  1  &  0.8736  & 0.21      \\ \hline
             min                 & 1      &  0.575  &  0.83   & 0.11  \\ \hline
             max                 & 1      &  0.7406     &  0.6420     & 0.2742      \\ \hline
             Sum-surplus         & 1      &  0.3448     &  0.5737     & 0.2006      \\ \hline
             Weight Density      & 1      &  0.4361     &  0.6834     & 0.1899      \\ \hline
             Balanced Density    & 1      &  0.2644        &  0.7133        & 0.0597      \\ \hline

        \end{tabular}
        \caption{The NDCG of different aggregate functions on DomainPub when $k = 6, r = 20, \epsilon = 0.8$.}
        \label{tab:dagg_ndcg}
    \end{table}

    \begin{table}[htbp]
        \centering
        \begin{tabular}{|c|c|c|c|c|} \hline
            \diagbox{functions}{methods} &  exact     & improved      & greedy     & random  \\ \hline
             avg                 & 4.32   &  1.92     &  0.58     & 0.58      \\ \hline
             sum                 & 0.347   &  0.054    &  0.024     & 0.026      \\ \hline
             min                 & 4.26   &  1.9     &  0.58      & 0.58      \\ \hline
             max                 & 4.25      &  1.88 &  0.59        & 0.58      \\ \hline
             Sum-surplus         & 4.28      &  1.91        &  0.58        & 0.58      \\ \hline
             Weight Density      & 4.26      &  1.88    &  0.58        & 0.58      \\ \hline
             Balanced Density    & 4.3      &  1.67        &  0.59        & 0.59      \\ \hline

        \end{tabular}
        \caption{The runtime of different aggregate functions on DomainPub when $k = 6, r = 20,  \epsilon = 0.8$.}
        \label{tab:dagg_runtime}
    \end{table}

\rev{A summary would be given for those parameters and some guidance would be given.}

\rev{\noindent \textbf{Summary of Parameters.}~Since there are several parameters, we discuss how to select these parameters. As for $\epsilon$, $0.1$ is feasible for most cases. When $\epsilon$ increases, the quality of result would decrease with a shorter runtime. As for $k$ and $r$, $k = 6$ and $r = 20$ are suitable for most cases. The trend of these two parameters is similar to that of $\epsilon$. It would be same for $s$, which suggested to be $20$ in these datasets.}

\begin{example}
\rev{Figure~\ref{fig:alg_exam} illustrates how Algorithm 2 and 3 runs and the intuition and the efficiency of Algorithm 3. Note that the aggregate function here is $sum$ and the number in each vertex is the influence value. $L$ is the set of the disjoint connected components after core decomposition. As for Algorithm 2, it needs to traverse all the possible candidates (the number of candidates is $5$ in this example, but could be large in real graph) and output the exact top $4$ result. The influence value of the first element in result set in Figure~\ref{ex_alg2} equals to $1+5+6+7=19$. Thus, the top $4$ influence values of results are $19, 18, 14, 13$. Nevertheless, for Algorithm $3$, we only need to traverse the feasible results set. As shown in Figure~\ref{ex_alg3}, the top $1$ influence value is $19$, $LB$ would be $19 \times (1-\epsilon) = 11.4$. Then, if any $4$ results with influence values larger than $11.4$ would terminate the algorithm.} 
\end{example}

% \begin{figure}[!t]
% 	\centering
% 	\begin{subfigure}[t]{0.15\textwidth}
% 		\centering
% 		\includegraphics[width=2.2cm]{figures/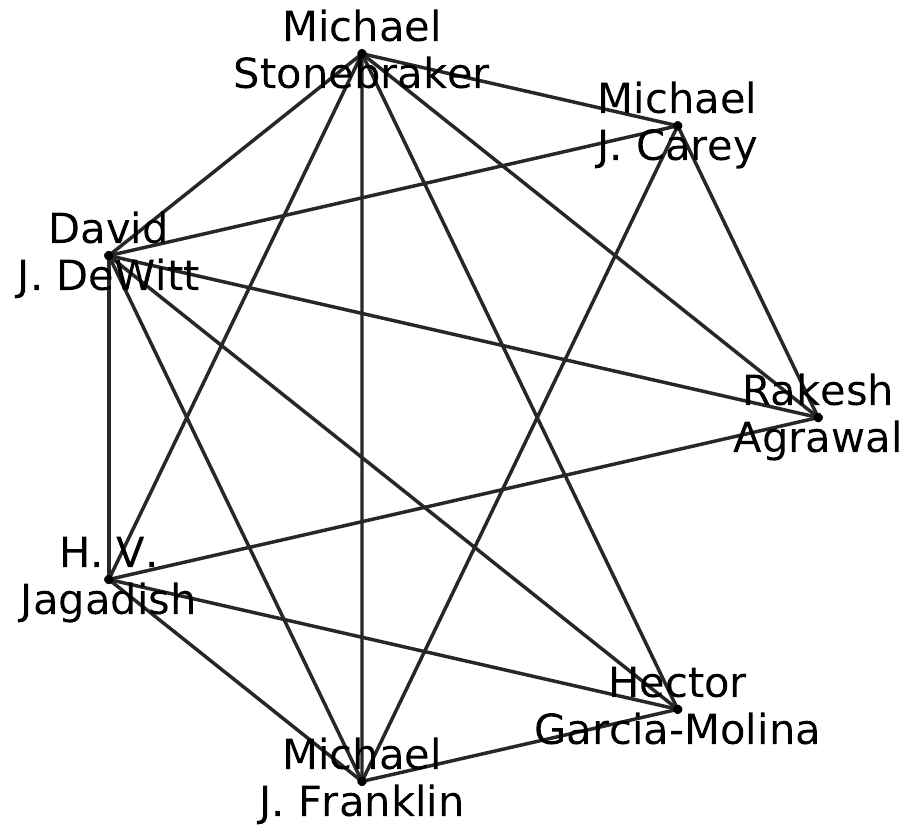}
% 		\caption{Min: top-$1$}
% 	\end{subfigure}%
% 	\begin{subfigure}[t]{0.15\textwidth}
% 		\centering
% 		\includegraphics[width=2.2cm]{figures/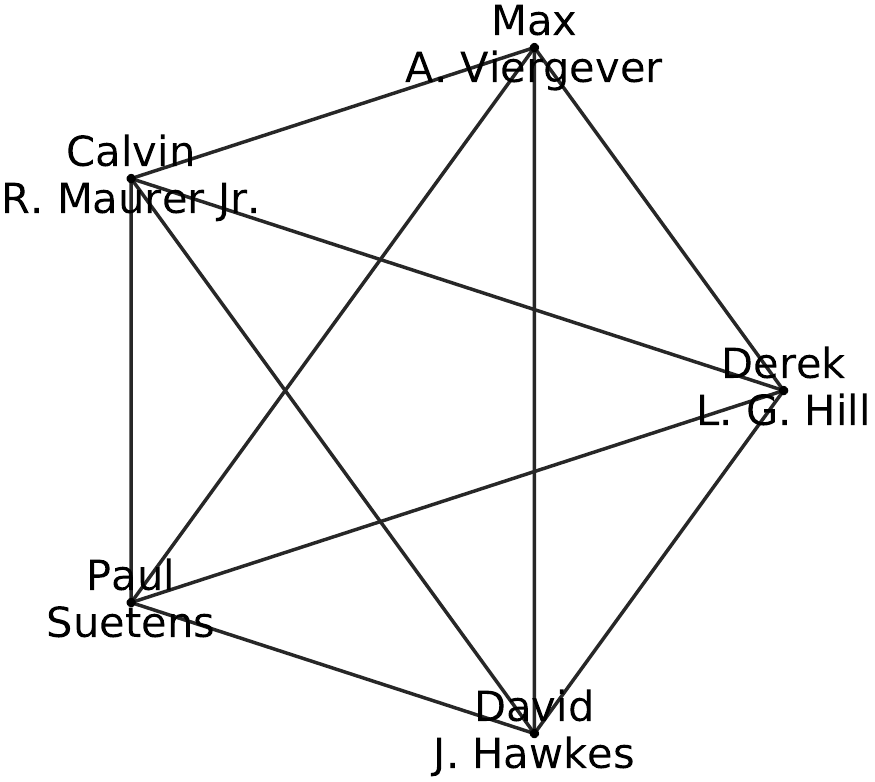}
% 		\caption{Min: top-$2$}
% 	\end{subfigure}%
% 	\begin{subfigure}[t]{0.15\textwidth}
% 		\centering
% 		\includegraphics[width=2.2cm]{figures/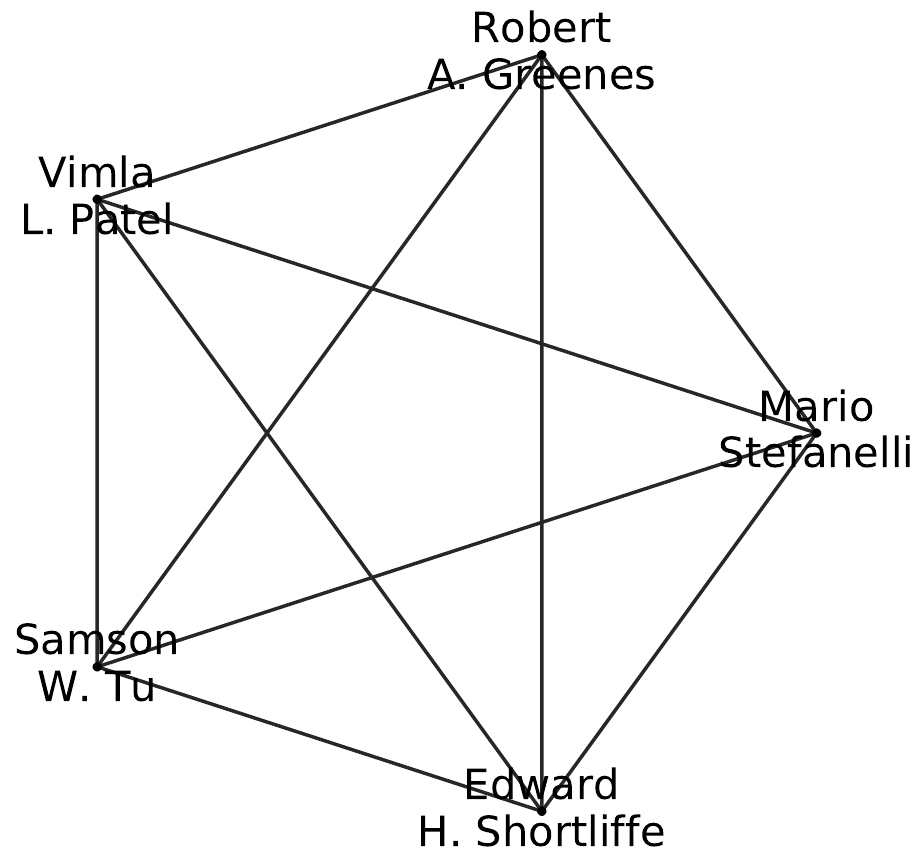}
% 		\caption{Min: top-$3$}
% 	\end{subfigure}%
	
% 	\begin{subfigure}[t]{0.15\textwidth}
% 		\centering
% 		\includegraphics[width=2.5cm]{figures/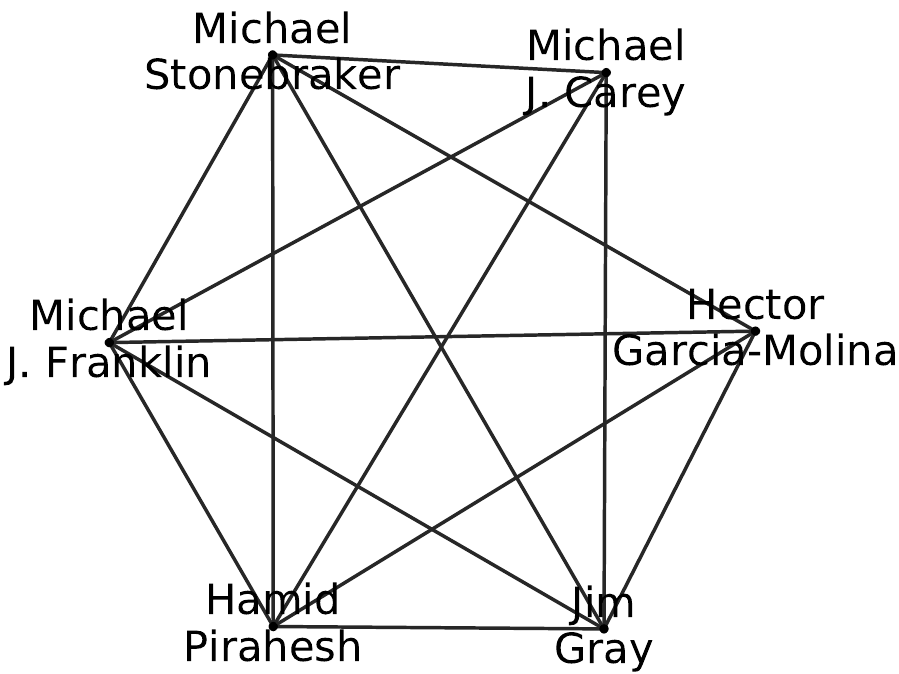}
% 		\caption{Avg: top-$1$}
% 	\end{subfigure}%
% 	\begin{subfigure}[t]{0.15\textwidth}
% 		\centering
% 		\includegraphics[width=2.5cm]{figures/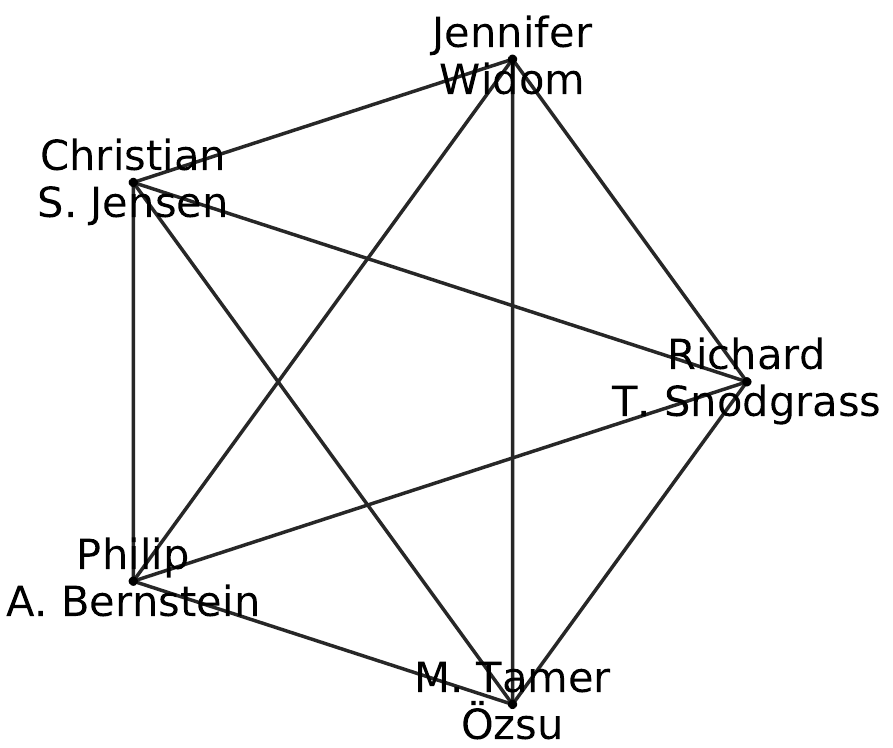}
% 		\caption{Avg: top-$2$}
% 	\end{subfigure}%
% 	\begin{subfigure}[t]{0.15\textwidth}
% 		\centering
% 		\includegraphics[width=2.2cm]{figures/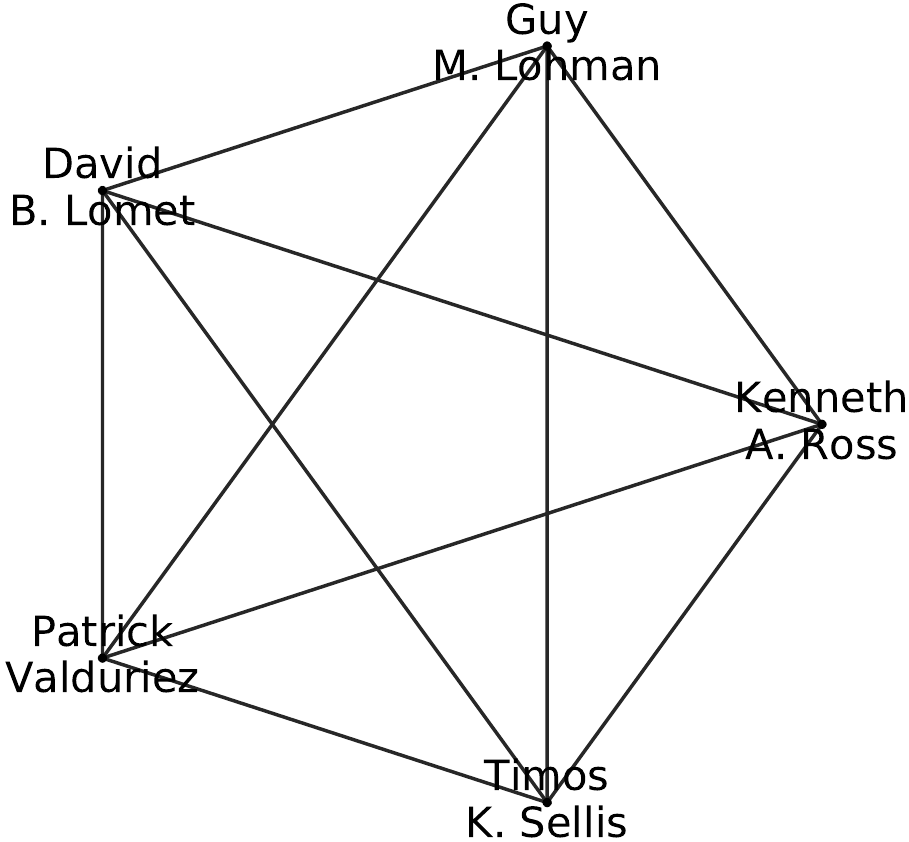}
% 		\caption{Avg: top-$3$}
% 	\end{subfigure}%
	
% 	\begin{subfigure}[t]{0.15\textwidth}
% 		\centering
% 		\includegraphics[width=2.5cm]{figures/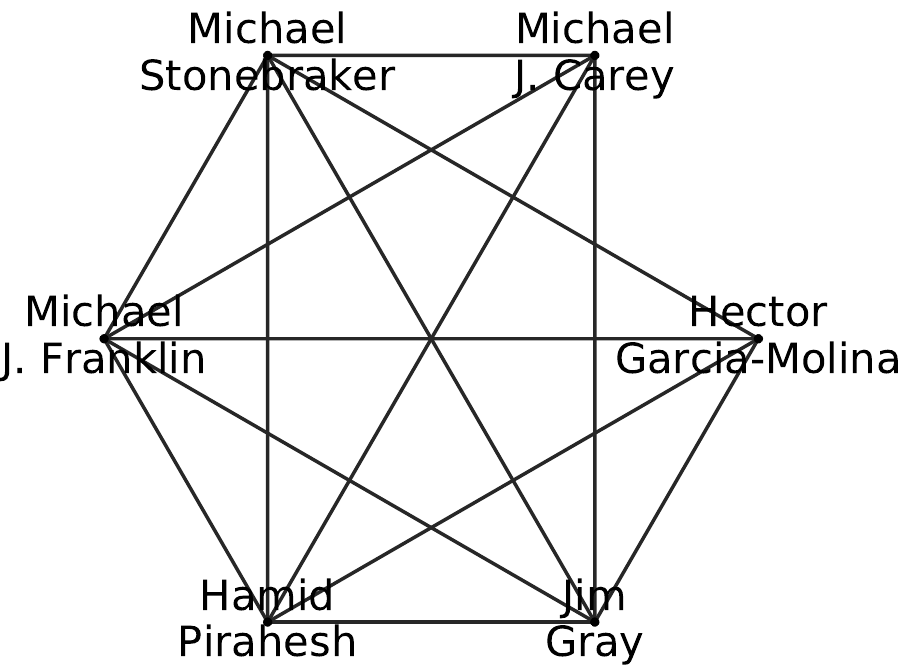}
% 		\caption{Sum: top-$1$}
% 	\end{subfigure}%
% 	\begin{subfigure}[t]{0.15\textwidth}
% 		\centering
% 		\includegraphics[width=2.5cm]{figures/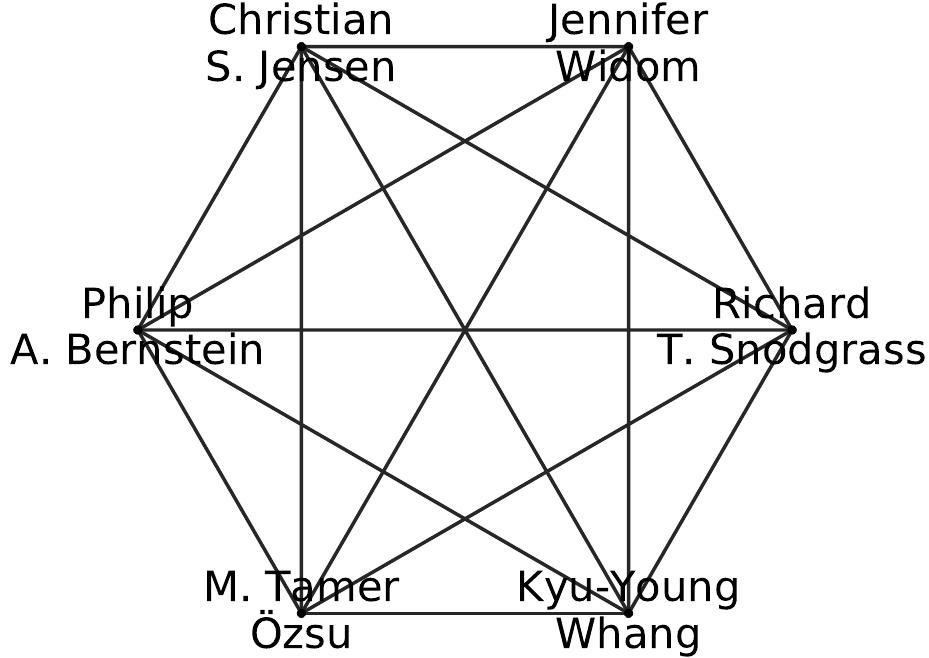}
% 		\caption{Sum: top-$2$}
% 	\end{subfigure}%
% 	\begin{subfigure}[t]{0.15\textwidth}
% 		\centering
% 		\includegraphics[width=2.5cm]{figures/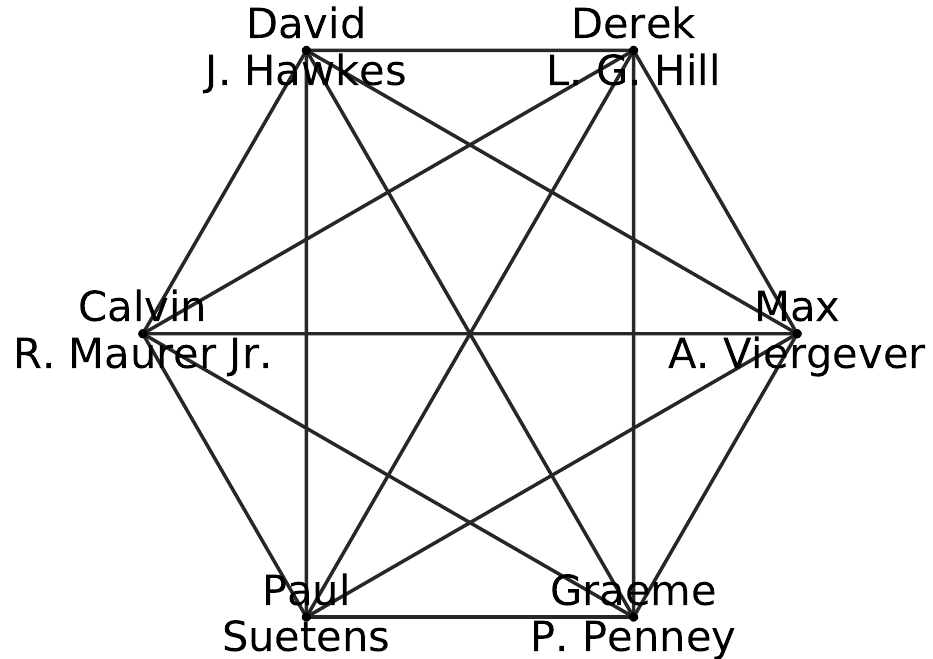}
% 		\caption{Sum: top-$3$}
% 	\end{subfigure}%
% 	\caption{Case Study: Aminer}
% 	\label{fig:case study}
% \end{figure}

\begin{figure}[htbp]
	\begin{center}
		\begin{subfigure}[t]{0.50\textwidth}
			\centering
			\includegraphics[scale=0.60]{figures/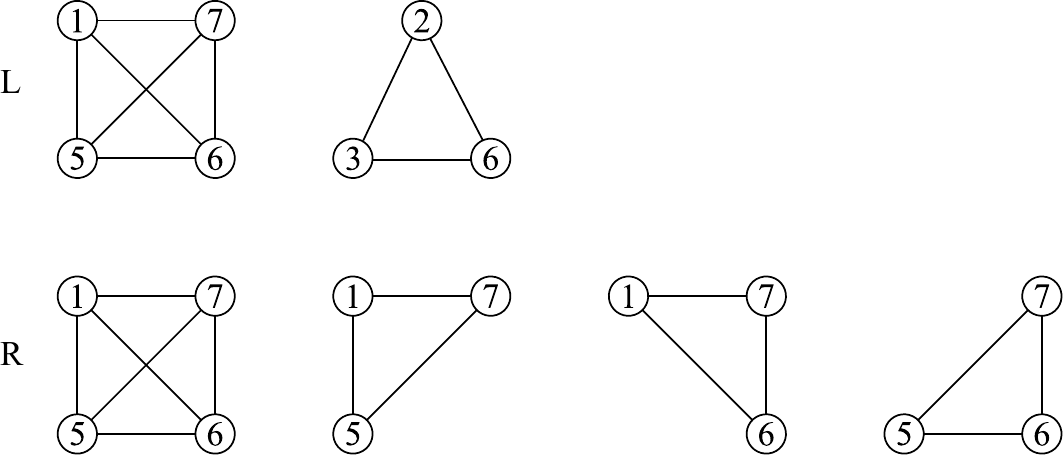}
					\caption{Algorithm 2 when $k=2$, $r=4$}
			\label{ex_alg2}
		\hspace{-10mm}
		\end{subfigure}
		\begin{subfigure}[t]{0.5\textwidth}
			\centering
			\includegraphics[scale=0.60]{figures/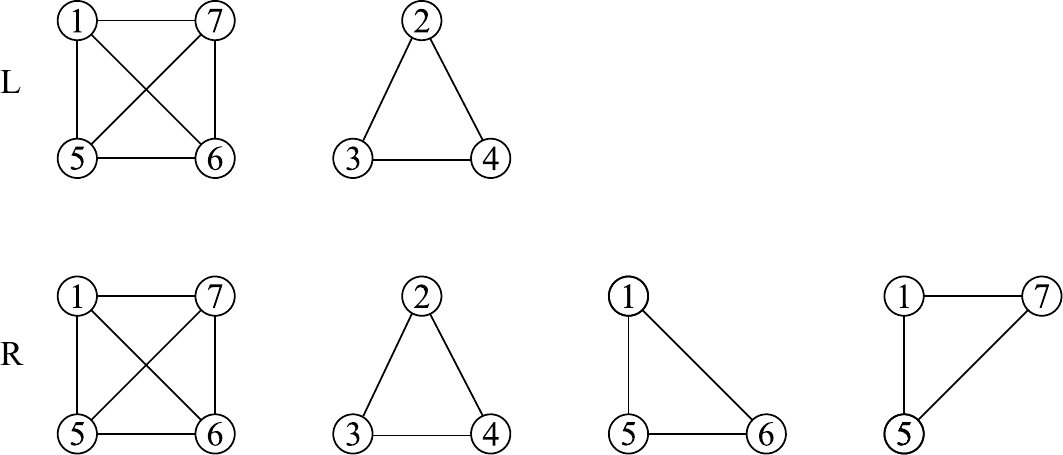}
		\caption{Algorithm 3 when $k=2$, $r=4$, and $\epsilon = 0.4$}
			\label{ex_alg3}
		\hspace{-10mm}
		\end{subfigure}
		
	\end{center}
	\vspace{-5mm}
	\caption{An example for how Algorithms 2 and 3 run} 
	\label{fig:alg_exam}
	\vspace{-3mm}
\end{figure}

        \begin{table}[htbp]
        \centering
        \begin{tabular}{|c|c|c|c|c|c|} \hline
\diagbox{$|V|$}{$\gamma$} &  2.1   & 2.2      & 2.3     & 2.4     & 2.5  \\ \hline
             50,000       & 0.05   &  0.03    &  0.03   & 0.03    & 0.02     \\ \hline
             100,000      & 0.08   &  0.07    &  0.07   & 0.05    & 0.05 \\ \hline
             150,000      & 0.14   &  0.12    &  0.1    & 0.09    & 0.08 \\ \hline
             200,000      & 0.2    &  0.17    &  0.15   & 0.13    & 0.11   \\ \hline
             250,000      & 0.26   &  0.22    &  0.19   & 0.17    & 0.16  \\ \hline
        \end{tabular}
        \caption{The runtime (second) of Algorithm 3 on Power-Law synthetic graphs when $k = 6, r = 20, \epsilon = 0.1$.}
        \label{tab:runtime_pl}
    \end{table}
    \rev{\textit{\textbf{Experiments on Power-Law Graphs.}~In this experiment, we evaluate the runtime by varying the $\gamma$ and $| V |$. It is illustrated in Table~\ref{tab:runtime_pl} that when the $\gamma$ increases, the runtime of Algorithm would decrease. This satisfies the time complexity analysis after Lemma 1.}}

\begin{table}[!t]
	\centering
	\begin{small}
		
		\caption{Submodular and Monotonic for different Aggregation Functions}
		\vspace{-2mm}
		\label{table:metrics}
		\begin{tabular}{|c|c|c|} \hline
			\cellcolor{gray!25}\textbf{Aggregation functions} & \cellcolor{gray!25}\textbf{Submodular} $f(H)$ & \cellcolor{gray!25}\textbf{Monotonic} \\ \hline
			Minimum &  \XSolid & \Checkmark \\ \hline
			Maximum &  \Checkmark & \Checkmark \\ \hline
			Sum & \Checkmark & \Checkmark \\ \hline
			Sum-surplus & \Checkmark & \Checkmark \\ \hline
			Average & \XSolid & \XSolid \\ \hline
			Weight Density & \XSolid& \Checkmark \\ \hline
			Balanced Density & \XSolid & \XSolid \\ \hline
		\end{tabular}
		\vspace{-2mm}
	\end{small}
\end{table}

\subsection{Proof for NP-hardness}
\rev{Here, we present the proofs to show when the aggregation function is weight density and balanced density.}

\begin{theorem}\label{thm:weight_density_topr}
\rev{When \fx is weight density, the top-$r$ $k$-influential community search problem is NP-hard.}
\end{theorem}

\begin{proof}
\rev{First, we set $\beta = 1$ here to show that there does not exist any algorithm could solve the top-$r$ $k$-influential community search problem in polynomial time when the aggregation function is weight density and $\beta = 1$. Given a graph $G=(V,E,w)$, we assign each vertex $v_i \in V$ with weight $0$. Then, we build another graph $G'=(V',E',w')$ by adding a new vertex $u$ that connects all vertices in $V$. We set the weight of the new vertex $u$ as $w_c$. Suppose that there exists a polynomial-time algorithm to address the top-$r$ $k$-influential community search problem. Then, we could determine whether there exists a ($k$-$1$)-clique since the influence value of top-$1$ $k$-influential community is $w_{c} - k$ if there exists a ($k$-$1$)-clique in graph $G$. Notably, adding any new vertex (or vertices) into such a clique would only increase the denominator of the influence value. However, the decision version of maximum clique search problem is NP-complete. It is a contradiction. Thus, top-$r$ $k$-influential community search problem is NP-hard, when \fx is weight density.}
\end{proof}

\begin{theorem}\label{thm:balanced_density_topr}
\rev{When \fx is balanced density, the top-$r$ $k$-influential community search problem is NP-hard.}
\end{theorem}

\begin{proof}
\rev{Given a graph $G=(V,E,w)$, we assign each vertex $v_i \in V$ with weight $1$ and $|V|=n$. Then, we build another graph $G'=(V',E',w')$ by adding a new vertex $u$ that connects all vertices in $V$. We set the weight of the new vertex $u$ as $w_c$. Suppose that there exists a polynomial-time algorithm to address the top-$r$ $k$-influential community search problem. Then, we could determine whether there exists a ($\lceil \frac{n-w_{c}}{2} \rceil$-$1$)-clique since the influence value of top-$1$ $k$-influential community is $(w_c + k) / (w_{c} + 2k -n)$, where $k = \lceil \frac{n-w_{c}}{2} \rceil$, if there exists a ($\lceil \frac{n-w_{c}}{2} \rceil$-$1$)-clique in graph $G$. Notably, adding any new vertex (or vertices) into such a clique would only increase the denominator of the influence value. However, the decision version of maximum clique search problem is NP-complete. It is a contradiction. Thus, top-$r$ $k$-influential community search problem is NP-hard, when \fx is balanced density.}
\end{proof}

% \begin{figure}[htbp]
% 	\begin{center}
% 		\includegraphics{\includegraphics[height=45mm]{figures/icde_example_alg2.pdf}}%\hspace{-10mm}
% 				\label{ex_alg2}
% 							\caption{Algorithm 2 when $k=2$, $r=4$}

% 			\label{ex_alg3}
% 			%\centering
% 			\includegraphics[height=45mm]{figures/icde_example_alg3.pdf}
% 					\caption[Algorithm 3 when $k=2$, $r=4$, and $\epsilon = 0.4$]{

% 		}%\hspace{-10mm}
% 	\end{center}
% 	\vspace{-5mm}
% 	\caption{An example for how Algorithms 2 and 3 run} 
% 	\label{fig:alg_exam}
% 	\vspace{-3mm}
% \end{figure}

% \begin{figure}[!htbp]
% 	\vspace{-2mm}
% 	\centering
% 	\includegraphics[height=45mm]{figures/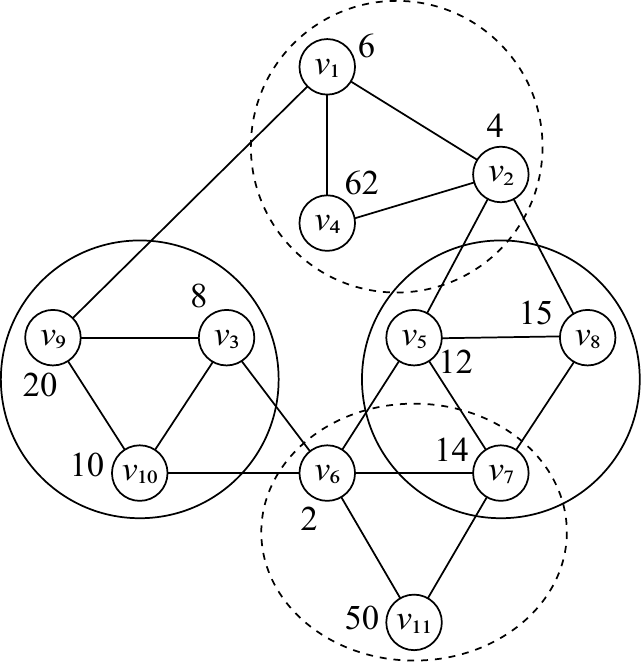}
% 	%	\vspace{-2mm}
% 	\caption{An example network}
% 	\label{fig:example}
% 	\vspace{-2mm}
% \end{figure}
